# Supplementary material for: New efficient algorithms for multiple change-point detection with kernels
Source: arXiv:1710.04556 source file (2017-10-12)
Supplement: Supplementary file 1 [file appendix.tex]

%%--------------------------------------------------
%%--------------------------------------------------
\appendix
\section*{Appendix}
\section{ Loss of a segmentation $m$ in $d$ segments}
\label{sec:loss-segm}
\begin{eqnarray}
 \Vert \mathrm{Y}-\hat{\mu}_{m_{d}}\Vert^2_{\mathcal{H}^n} &= & \Vert \mathrm{Y} \Vert^2_{\mathcal{H}^n} + \Vert \hat{\mu}_{m_{d}}\Vert^2_{\mathcal{H}^n} - 2\langle \mathrm{Y},  \hat{\mu}_{m_{d}} \rangle_{\mathcal{H}^n} \nonumber
\end{eqnarray}

Let computing separately each terms : 
\begin{eqnarray}
 \Vert \mathrm{Y} \Vert^2_{\mathcal{H}^n}  &= & \displaystyle \sum_{t = 1}^{n}  \Vert \mathrm{Y}_t \Vert^2_{\mathcal{H}}  = \displaystyle \sum_{t = 1}^{n} \langle \mathrm{Y}_t,\mathrm{Y}_t\rangle_{\mathcal{H}} = \displaystyle \sum_{t = 1}^{n} \langle \Phi(\mathrm{X}_t),\Phi(\mathrm{X}_t)\rangle_{\mathcal{H}}\nonumber\\
 & =& \displaystyle \sum_{t = 1}^{n} k( \mathrm{X}_t,\mathrm{X}_t)
\end{eqnarray}

\begin{eqnarray}
\Vert \hat{\mu}_{m_{d}}\Vert^2_{\mathcal{H}^n}  & = & \displaystyle \sum_{t = 1}^{n} \Vert \hat{\mu}_{m_{d}}(t)\Vert^2_{\mathcal{H}} = \displaystyle \sum_{t = 1}^{n} \langle \hat{\mu}_{m_{d}}(t),\hat{\mu}_{m_{d}}(t)\rangle_{\mathcal{H}} \nonumber\\
&=& \displaystyle \sum_{t = 1}^{n} \langle  \frac{1}{n_{\lambda(t)}}\sum_{j\in \lambda(t)} \mathrm{Y}_j, \frac{1}{n_{\lambda(t)}}\sum_{l\in \lambda(t)} \mathrm{Y}_l\rangle_{\mathcal{H}} \nonumber\\
&=& \sum_{t = 1}^{n} \frac{1}{n_{\lambda(t)}^2}\sum_{j\in \lambda(t)}\sum_{l\in \lambda(t)}  \langle  \mathrm{Y}_j, \mathrm{Y}_l\rangle_{\mathcal{H}} =\displaystyle \sum_{\lambda\in m_{d}} \frac{n_{\lambda}}{n_{\lambda}^2} \sum_{j,l\in \lambda}\langle  \mathrm{Y}_j, \mathrm{Y}_l\rangle_{\mathcal{H}}\nonumber\\
&=& \displaystyle \sum_{\lambda\in m_{d}} \frac{1}{n_{\lambda}} \sum_{j,l\in \lambda}k(\mathrm{X}_j, \mathrm{X}_l)
\label{eq:normMuHat}
\end{eqnarray}
\text{ where $\lambda(t)$ of segmentation $m_d$ is the unique segment which contain element $t$} 
\begin{eqnarray}
\langle \mathrm{Y},  \hat{\mu}_{m_{d}} \rangle_{\mathcal{H}^n} &  = & \displaystyle \sum_{t = 1}^{n} \langle \mathrm{Y}_t, \hat{\mu}_{m_d}(t)\rangle_{\mathcal{H}} =  \sum_{t = 1}^{n} \langle \mathrm{Y}_t, \frac{1}{n_{\lambda(t)}} \sum_{j\in \lambda(t)}\mathrm{Y_j}\rangle_{\mathcal{H}}\nonumber\\
&=&  \sum_{t = 1}^{n} \frac{1}{n_{\lambda(t)}} \sum_{j\in \lambda(t)}\langle \mathrm{Y}_t,  \mathrm{Y_j}\rangle_{\mathcal{H}}= \displaystyle \sum_{\lambda \in m_{d} } \frac{1}{n_{\lambda}} \sum_{l,j\in \lambda}\langle \mathrm{Y}_l,  \mathrm{Y_j}\rangle_{\mathcal{H}}\nonumber\\
&=&\displaystyle \sum_{\lambda \in m_{d} } \frac{1}{n_{\lambda}} \sum_{l,j\in \lambda}k(\mathrm{X}_l,  \mathrm{X_j})
\label{eq:scalmuHatY}
\end{eqnarray}
\text{ where $\lambda(t)$ of segmentation $m_d$ is the unique segment which contain element $t$} 

We notice that elements \ref{eq:normMuHat} and \ref{eq:scalmuHatY} are equal and hence,
\begin{eqnarray}
 \Vert \mathrm{Y}-\hat{\mu}_{m_{d}}\Vert^2_{\mathcal{H}^n} &= & \Vert \mathrm{Y} \Vert^2_{\mathcal{H}^n} - \Vert \hat{\mu}_{m_{d}}\Vert^2_{\mathcal{H}^n}\nonumber\\
 &=& \displaystyle \sum_{t = 1}^{n} k( \mathrm{X}_t,\mathrm{X}_t)-\displaystyle \sum_{\lambda \in m_{d} } \frac{1}{n_{\lambda}} \sum_{l,j\in \lambda}k(\mathrm{X}_l,  \mathrm{X_j})\nonumber
\end{eqnarray}

To conclude:

\begin{eqnarray}
\hat{m}_d = \displaystyle \argmin_{m_d\in\mathcal{M}_n(d)} \sum_{t=1}^n k(\mathrm{X}_t,\mathrm{X}_t) - \sum_{\lambda\in m_d} \frac{1}{n_{\lambda}}\sum_{l,j\in \lambda}k(\mathrm{X}_l,\mathrm{X}_j)
\end{eqnarray}

\section{Performance on allele B fraction dimension}
\label{sec:performance-allele-b}
Let denote $\mathrm{I}(i,j)$ the integral of product between Gaussian densities $\mathcal{N}(\nu_i,\gamma_i^2)$ and  $\mathcal{N}(\nu_j,\gamma_j^2)$ :
\begin{eqnarray}
\mathrm{I}(i,j)&=&\int_{\mathds{R}} f_i(x)f_j(x)dx\nonumber\\
& = &\int_{\mathds{R}} \frac{1}{\sqrt{2\pi \gamma_i^2}}\exp\left(-\frac{1}{2} \left(\frac{x-\nu_i}{\gamma_i}\right)^2\right)\frac{1}{\sqrt{2\pi \gamma_j^2}}\exp\left(-\frac{1}{2} \left(\frac{x-\nu_j}{\gamma_j}\right)^2\right)dx\nonumber\\
& = & \frac{1}{2\pi \gamma_i\gamma_j} \int_{\mathds{R}} \exp\left(- \left(\frac{(x-\nu_i)^2}{2\gamma_i^2} +\frac{(x-\nu_j)^2}{2\gamma_j^2}\right)\right)dx\nonumber\\
& = & \frac{1}{2\pi \gamma_i\gamma_j} \int_{\mathds{R}} \exp\left(- \frac{1}{2\gamma_i^2\gamma_j^2}\left( x^2(\gamma_i^2+\gamma_j^2)+\nu_i^2\gamma_j^2+\nu_j^2\gamma_i^2-2x(\nu_i\gamma_j^2+\nu_j\gamma_i^2)\right)\right)dx\nonumber\\
& = & \frac{1}{2\pi \gamma_i\gamma_j} \int_{\mathds{R}} \exp\left(- \frac{\gamma_i^2+\gamma_j^2}{2\gamma_i^2\gamma_j^2}\left( x^2+\frac{\nu_i^2\gamma_j^2+\nu_j^2\gamma_i^2}{\gamma_i^2+\gamma_j^2}-2x\frac{(\nu_i\gamma_j^2+\nu_j\gamma_i^2)}{\gamma_i^2+\gamma_j^2}\right)\right)dx\nonumber\\
& = & \frac{1}{2\pi \gamma_i\gamma_j} 
\int_{\mathds{R}} \exp
\left(- \frac{\gamma_i^2+\gamma_j^2}{2\gamma_i^2\gamma_j^2}
		\left( 
				\left(x-\frac{\nu_i\gamma_j^2+\nu_j\gamma_i^2}{\gamma_i^2+\gamma_j^2}\right)\right.\right.+\nonumber\\
				&&\left.\left.
				\qquad\frac{\nu_i^2\gamma_j^2+\nu_j^2\gamma_i^2}{\gamma_i^2+\gamma_j^2}-
				\left(\frac{\nu_i\gamma_j^2+\nu_j\gamma_i^2}{\gamma_i^2+\gamma_j^2}\right)^2
		\right)
\right)dx\nonumber\\
\end{eqnarray}
Then, let :
\begin{itemize}
\item $a=\frac{\nu_i\gamma_j^2+\nu_j\gamma_i^2}{\gamma_i^2+\gamma_j^2}$
\item $b^2=\frac{\gamma_i^2\gamma_j^2}{\gamma_i^2+\gamma_j^2}$
\item $c=\frac{\nu_i^2\gamma_j^2+\nu_j^2\gamma_i^2}{\gamma_i^2+\gamma_j^2}-
				\left(\frac{\nu_i\gamma_j^2+\nu_j\gamma_i^2}{\gamma_i^2+\gamma_j^2}\right)^2$
\end{itemize}
\begin{eqnarray}
\mathrm{I}(i,j)& = & \frac{1}{2\pi\gamma_i\gamma_j}\exp\left(-\frac{c}{2b^2}\right)\int_{\mathds{R}}\exp\left(-\frac{1}{2b^2}\left(x-a\right)^2\right)dx\nonumber\\
& = & \frac{\sqrt{2\pi b^2}}{2\pi\gamma_i\gamma_j}\exp\left(-\frac{c}{2b^2}\right)\int_{\mathds{R}}\frac{1}{\sqrt{2\pi b^2}}\exp\left(-\frac{1}{2b^2}\left(x-a\right)^2\right)dx\nonumber\\
& = & \frac{b}{\sqrt{2\pi}\gamma_i\gamma_j}\exp\left(-\frac{c}{2b^2}\right)\nonumber
\end{eqnarray}
To finish we replace by $c$ and $b$ by their expressions.
\begin{eqnarray}
\mathrm{I}(i,j)&=&\frac{1}{\sqrt{2\pi(\sigma^2_i+\sigma^2_j)}} \exp\left( - \frac{\nu_i\gamma_j^2+\nu_j\gamma_i^2-(\nu_i\gamma_j^2+\nu_j\gamma_i^2)/(\gamma_i^2+\gamma_j^2)}{2\gamma_i^2\gamma_j^2}\right)\nonumber
\label{eq:Int}
\end{eqnarray}

The estimation $\hat{f}_{\hat{m}}$ of $f^{\star}$ is computed with classical EM algorithm.\\
